# Supplementary material for: Differentiable Transient Rendering
Source: arXiv:2206.06193 source file (2022-06-13)
Supplement: Supplementary file 1 [file background-supple.tex]

\section{Mathematical Background}
In differentiable rendering, the image can be represented as an integral over an evolving manifold containing the path space, and s cene derivatives can be evaluated using transport theorems. For completeness, we introduce here the related mathematical background.
We will follow existing terminology and definitions of fluid and continuum mechanics~\cite{cermelli2005transport}, mathematics~\cite{seguin2014roughening}, and their application to differentiable rendering~\cite{zhang2020path}.

\subsection{Mathematical Notions}
We first add details of common concepts in mathematical analysis and differential geometry used in our work.

\paragraph{Open and closed sets}
A set in the Euclidean space $U \subset \R^n$ is called an \textit{open set} if for any $\bfx\in U$ there exists $\epsilon>0$ s.t. $\left\{\bfy\in \R^n\mid \norm{\bfy-\bfx}<\epsilon\right\}$ $\subset U$. A set $U \subset X \subset \R^n$ is called an \textit{open set relative to} $X$ if for any $\bfx\in U$ there exists $\epsilon>0$ s.t. $\left\{\bfy\in X\mid \norm{\bfy-\bfx}<\epsilon\right\}\subset U$. A set $A \subset \R^n$ (resp. $A \subset X\subset \R^n$) is called a \textit{closed set} (resp. \textit{closed set relative to} $X$) if $\R^n -A$ (resp. $X-A$) is an open set (resp. open set relative to $X$). 

\paragraph{Continuous functions}
For sets $X$ and $Y\subset \R^n$, a function $\varphi\colon X\to Y$ is called \textit{continuous} if for any open set $U$ relative to $Y$, $\varphi^{-1}\left(U\right)$ is open relative to $X$. Note that this definition is equivalent to the epsilon-delta argument.

\paragraph{Manifolds}
We define the halfspace as:
\begin{equation}
	\mathbb{H}^n \coloneqq\left\{ \left(x_1...x_n\right)\in \R^n\mid x_1 \ge 0\right\}.
\end{equation}
Then a set $\calM \subset \R^n$ is called an $m$-\textit{dimensional manifold} (or $m$-manifold) if for any $\bfx\in\mathcal{M}$ there exists an open set $U_{\bfx}$ relative to $\calM$ and a one-to-one function $\phi_{\bfx}\colon U_{\bfx}\to \phi_{\bfx}\left(U_{\bfx}\right)\subset \mathbb{H}^m$, called a chart, such that both $\phi_{\bfx}$ and $\phi_{\bfx}^{-1}$ are continuous. Note that if we can choose each chart $\phi_{\bfx}$ so that both $\phi_{\bfx}$ and $\phi_{\bfx}^{-1}$ are $C^i$-differentiable then $\calM$ is called a $C^i$-differentiable manifold. The \textit{boundary} (or boundary manifold) of $\calM$ is defined as:
\begin{equation}
	\label{eq:def_manibd}
	\partial\calM\coloneqq\left\{\bfx \in \calM\mid\ \text{the first coordinate of }\phi_{\bfx}\left(\bfx\right)\text{ is zero}\right\}.
\end{equation}
Note that this definition  is independent of the choice of a particular open set $U_{\bfx}$ and chart $\phi_{\bfx}$, and that $\partial\calM$ is a $(m-1)$-manifold. The \textit{interior} of $\calM$ is defined as $\Int\calM\coloneqq \calM-\partial\calM$.

We can intuitively understand an $m$-manifold $\calM$ as a set of space of points that need at least $m$ real numbers to parameterize all points in $\calM$. For instance, a surface mesh embedded in $\R^3$ is a $2$-manifold, and the space of light paths $\Omega_k$ with $k+1$ vertices is a $2\left(k+1\right)$-manifold embedded in $\R^{3\left(k+1\right)}$.

\paragraph{Tangent space}
Suppose that $\calM\subset \R^n$ is a $C^1$-differentiable $m$-manifold. The \textit{tangent space} of $\calM$ on $\bfx\in\calM$ is then defined as:
\begin{align}
	\begin{split}
		T_{\bfx}\calM \coloneqq \{ \dot\gamma\left(0\right) \mid &\gamma\colon \left(-\epsilon,\epsilon\right)\to\calM \text{ is a differentiable curve,}\\& \text{and }\gamma\left(0\right)=\bfx \}\subset\R^n,
	\end{split}
\end{align}
where the derivative (velocity w.r.t. parameterization) of the curve $\dot \gamma \left(0\right)$ can be evaluated as  usual  in $\R^n$. Note that $T_\bfx \calM$ is an $m$-dimensional vector space; a vector in $T_\bfx \calM$ is called a \textit{tangent vector}.

\subsection{Evolving Manifolds}

An \textit{evolving} $m$-\textit{manifold} $\calM\left(\btheta\right)\subset \R^n$ with respect to the \textit{scene parameter} $\btheta\in \R^d$ can be considered as a function mapping each value of the parameter $\btheta$ to each $m$-manifold. Its \textit{trajectory} is defined as $\calJ\coloneqq \left\{\left(\bfx,\btheta\right)\mid x\in \calM\left(\btheta\right), \btheta\in\R^d \right\} \subset \R^{n+d}$.
When $\calM\left(\btheta\right)$ evolves continuously, we can assume that $\calJ$ is an $\left(m+d\right)$-manifold. In the following we fix the scene parameters vector $\btheta=\left(\theta_1...\theta_d\right)$ as a single scalar $\theta$ for simplicity. Generalization to vector $\btheta$ will be introduced at the end of this section.

While we have the motion of the entire manifold $\calM$ with respect to $\theta$, describing the motion of a single point $\bfx\in\calM\left(\theta\right)$ cannot be defined in a trivial way. A \textit{local parameterization} is defined as a one-to-one function $\hat\bfx \colon U\to \calJ$ such that $U$ is open in $\R^{n}\times\R$ and $\hat\bfx\left(\bfp,\theta'\right)\in\calM\left(\theta'\right)$ for any $\left(\bfp,\theta'\right)\in U$. Suppose a local parameterization for a given point $\bfx\in\calM\left(\theta\right)$, i.e., there exists $\left(\bfp_0,\theta\right)\in U$ s.t. $\hat\bfx\left(\bfp_0,\theta\right)=\bfx$. Then we can define the \textit{local velocity} of $\bfx$ as:
\begin{equation}
	\label{eq:local_paramz}
	v\left(\bfx,\theta\right)\coloneqq
	\left.\pfrac{}{\theta'} \hat{\bfx}\left(\bfp_0,\theta'\right)\right|_{\theta'=\theta}\in \R^n.
\end{equation} 

The local velocity depends on the choice of local parameterization. Unlike fluid or continuum mechanics, we should eliminate this dependency to get well-defined formulations on evolving manifolds. When the codimenison of $\calM$ is one, i.e., $n=m+1$, the \textit{scalar normal velocity} $\calV_\calM\left(\bfx,\theta\right)$ and \textit{local tangential velocity} $v_{\mathrm{tan}}\left(\bfx,\theta\right)$ of a given point $\bfx\in\calM\left(\theta\right)$ are defined as:

\begin{gather}
	\label{eq:normvel}
	\calV_\calM \left(\bfx,\theta\right) \coloneqq v\left(\bfx,\theta\right) \cdot \bfn\left(x,\theta\right), \\
	\label{eq:tanvel}
	v_\mathrm{tan}\left(\bfx,\theta\right) \coloneqq v\left(\bfx,\theta\right) - \calV_\calM \left(x,\theta\right) \bfn \left(x,\theta\right),
\end{gather}
where $\bfn \left(x,\theta\right)$ denotes the unit normal vector of $\calM\left(\theta\right)$ at $\bfx$. Then the local tangential velocity $v_{\mathrm{tan}}\left(\bfx,\theta\right)$ still depends on the local parameterization, but the scalar normal velocity $\calV_\calM\left(\bfx,\theta\right)$ is independent of such local parameterization. However, while the surface geometry embedded in $\R^3$ has codimension one, the space of light paths $\Omega_k$ has a higher codimension $\left(k+1\right)$, so the normal vector $\bfn$ cannot be defined. Thus, more generally, the local tangential velocity and the \textit{vector normal velocity} $\vec{\calV}_\calM\left(\bfx,\theta\right)$ are defined as:

\begin{gather}
	\label{eq:tanvel2}
	v_\mathrm{tan}\left(\bfx,\theta\right) \coloneqq \Pi_{T_\bfx \calM}\left(v\left(\bfx,\theta\right)\right), \\
	\label{eq:normvel2}
	\vec{\calV}_\calM\left(\bfx,\theta\right) \coloneqq v\left(\bfx,\theta\right) - v_\mathrm{tan}\left(\bfx,\theta\right),
\end{gather}
where $\Pi_{T_\bfx \calM} \colon \R^n \to T_\bfx \calM$ denotes the canonical projection (orthogonal projection) from a vector space onto a subspace. Note that the definitions of $v_\mathrm{tan}$ in Equations~\eqref{eq:tanvel} and \eqref{eq:tanvel2} are equivalent, while  $\calV_\calM$ in Equation~\eqref{eq:normvel} and $\vec{\calV}_\calM$ in Equation~\eqref{eq:normvel2} are related as $\vec{\calV}_\calM=\calV_\calM \bfn$ when $n=m+1$. Steady-state path-space differentiable rendering~\cite{zhang2020path} did not use the vector normal velocity since the authors relied on the Reynolds transport relation on a 2D manifold embedded in $\R^3$. This is no longer possible in transient state, an thus the need to apply the generalized transport theorem on the path space $\Omega_k\subset\R^{3\left(k+1\right)}$.

The boundary of the evolving manifold, $\partial\calM\left(\theta\right)$, is also an evolving manifold. We can define a local velocity $v_{\partial\calM}\left(\bfx,\theta\right)$, a local tangential velocity $v_{\mathrm{tan},\partial\calM}\left(\bfx,\theta\right)$, and a vector normal velocity $\vec{\calV}_{\partial \calM}\left(\bfx,\theta\right)$ on $\partial\calM\left(\theta\right)$ in the same fashion, but the scalar normal velocity $\calV_{\partial\calM}\left(\bfx,\theta\right)$ at $\bfx\in\partial\calM\left(\theta\right)$ is defined differently as:
\begin{gather}
	\label{eq:bd_normal_velocity}
	v_{\mathrm{tan},\partial\calM}\left(\bfx,\theta\right) \coloneqq \Pi_{T_{\bfx} \partial\calM}\left(v_{\partial\calM}\left(\bfx,\theta\right)\right), \\
	\vec{\calV}_{\partial\calM}\left(\bfx,\theta\right) \coloneqq v_{\partial\calM}\left(\bfx,\theta\right) - v_{\mathrm{tan},\partial\calM}\left(\bfx,\theta\right),\\
	\calV_{\partial\calM}\left(\bfx,\theta\right) \coloneqq \vec{\calV}_{\partial\calM}\left(\bfx,\theta\right)\cdot \bfn_{\partial\calM}\left(\bfx,\theta\right),
\end{gather}
where $\bfn_{\partial\calM}\left(\bfx,\theta\right)\in T_{\bfx}\calM\left(\theta\right)$. Note that when restricting the direction of the unit normal vector $\bfn_{\partial\calM}\left(\bfx,\theta\right)$ into $T_{\bfx}\calM\left(\theta\right)$ (instead of into $\R^n$) the outgoing normal direction $\bfn_{\partial\calM}$ from $\calM\left(\theta\right)$ is determined uniquely, so that we can use the scalar normal velocity of $\partial\calM\left(\theta\right)$ under the general dimensionality of $\calM\left(\theta\right)$ and $\R^n$.

\subsection{Generalized Transport Theorem for Evolving Manifolds}

Suppose that there is a scalar field $\varphi\colon\mathcal{J}\to \R$ defined on an evolving manifold. Generally, the field $\varphi$ could not be defined on the entire space $\R^{n+1}$, so the partial derivative of the field $\varphi$ with respect to $\theta$ cannot be defined in a trivial way. In other words, when trying to evaluate $\lim_{\epsilon\to 0} \frac{\varphi\left(\bfx,\theta+\epsilon\right)-\varphi\left(\bfx,\theta\right)}{\epsilon}$, the numerator cannot be defined unless $\bfx$ lies on both  $\calM\left(\theta\right)$ and $\calM\left(\theta+\epsilon\right)$. Therefore, we first define a derivative which depends on the choice of local parameterization, then we can define a parameterization-independent derivative from the dependent one.
The \textit{derivative} $\dot\varphi\left(\bfx,\theta\right)$ w.r.t. $\theta$, which depends on choice of local parameterization, and the \textit{normal derivative} $\varphi^\square \left(\bfx,\theta\right)$ w.r.t. $\theta$, which is independent of local parameterization, are defined as follows:
\begin{gather}
	\label{eq:derivative_field}
	\dot\varphi\left(\bfx,\theta\right) \coloneqq \left. \pfrac{}{\theta'} \varphi\left(\hat{\bfx}\left(\bfp_0,\theta'\right),\theta'\right) \right|_{\theta'=\theta}, \\
	\overset{\square}{\varphi}\left(\bfx,\theta\right) \coloneqq \dot\varphi\left(\bfx,\theta\right) - v_\mathrm{tan}\left(\bfx,\theta\right) \cdot \mathrm{grad}_\calM \varphi\left(\bfx,\theta\right).
\end{gather}

Now we investigate the derivative of the integration over evolving manifolds. Seguin et al.~\shortcite{seguin2014roughening}  showed that the derivative of the integral of $\varphi$ over the evolving manifold $\calM\left(\theta\right)$ can be represented as the \textit{transport theorem for evolving manifolds}:

\begin{equation}
	\label{eq:diffint_evol_man}\small
	\dfrac{}{\theta} \int_{\calM\left(\theta\right)}{\varphi \d \mu_\calM } = \int_{\calM\left(\theta\right)} { \left(\overset{\square}{\varphi} - \varphi\vec{\kappa} \cdot \vec{\calV}_\calM\right) \d \mu_\calM}	
	+ \int_{\partial\calM\left(\theta\right)} { \varphi \calV_{\partial \calM} \d \mu_{\partial\calM} },
\end{equation}
where $\vec\kappa$ is the \textit{total curvature vector},  $m$ times the mean curvature vector on the $m$-manifold $\calM\left(\theta\right)$, and $\mu_\calM$ and $\mu_{\partial\calM}$ are the measures on $\calM\left(\theta\right)$ and $\partial\calM\left(\theta\right)$, respectively. The mean curvature vector on a $m$-manifold embedded in $\R^n$ has been defined in differential geometry \cite{carmo1992riemannian,chen1975mean}. According to their definition, the mean curvature vectors can be well defined for arbitrary codimensions, i.e., even if $n > m+1$, so that the unit normal vector on the manifold is not uniquely defined.

Note that this transport theorem has been given different names depending on the dimension $m$ and the codimension $n$. For the simplest case, $m=n=1$, the theorem is called the Leibniz integral rule, and for the case of $m=n=3$ (or any case of $m=n$) the theorem is usually called the Reynolds transport theorem. Zhang et al.~\shortcite{zhang2020path}  used this transport theorem for the particular case of $m=2$ and $n=3$, and applied it iteratively. Our work generalizes this for any dimension and codimension.

\subsection{Generalized Transport Theorem with Discontinuity}
\label{sec:transport_theorem_disconti}
In this section we will treat the case when the scalar field $\varphi$ contains discontinuities. For simplicity, our notations follow previous work~\cite{zhang2020path}. The \textit{discontinuity set} (discontinuity submanifold) of $\calM\left(\theta\right)$ with respect to $\varphi$ is defined as:
\begin{equation}
	\label{disconti_submani}
	\Delta\calM\left[\varphi\right]\left(\theta\right)\coloneqq\left\{ \bfx\in\calM\left(\theta\right) \mid \varphi\left(\cdot,\theta\right)\text{ is discontinuous at }\bfx\right\}.
\end{equation}
We assume that $\Delta\calM\left[\varphi\right]\left(\theta\right)$ can be represented as a finite union of $(m-1)$-submanifolds of $\calM\left(\theta\right)$, and that $\Delta\calM\left[\varphi\right]\left(\theta\right)$ itself evolves continuously. Then the \textit{continuous interior} $\Intc \calM\left[\varphi\right]\left(\theta\right)$ and the \textit{extended boundary} $\exbdM\left[\varphi\right]\left(\theta\right)$ of $\calM$ with respect to $\varphi$ are defined as follows:
\begin{align}
	\begin{split}
	\label{eq:def_contiint}	
	\Intc \calM\left[\varphi\right]\left(\theta\right) \coloneqq& \Int \calM \left(\theta\right) - \Delta\calM\left[\varphi\right]\left(\theta\right) \\=& \calM\left(\theta\right)-\partial\calM\left(\theta\right)-\Delta\calM\left[\varphi\right]\left(\theta\right),
	\end{split}
\\
	\begin{split}
		\label{eq:def_exbd}
		\exbdM\left[\varphi\right]\left(\theta\right) \coloneqq& \partial\calM\left(\theta\right)\cup \Delta\calM\left[\varphi\right]\left(\theta\right).
	\end{split}
\end{align}
Note that when $\calM$ is a 2D manifold (surface), $\Delta\calM$ can also be called a discontinuity \textit{curve}, as in Zhang et al.~\shortcite{zhang2020path}. We will often omit the dependency $\left[\varphi\right]$ or $\left(\theta\right)$ for simplicity.

The scalar field $\varphi$ is continuous on each connected component of the continuous interior $\Intc\calM$, so the integral over $\calM$ can be represented as the sum of integrals over each connected component of $\Intc\calM$. Then we can apply the transport theorem~\eqref{eq:diffint_evol_man} for each connected component, and finally obtain the transport theorem with discontinuities:

\begin{equation}
	\label{eq:trans_thm_discont}
	\dfrac{}{\theta} \int_{\calM\left(\theta\right)}{\varphi \d \mu_\calM}
	= \int_{\calM} { \left(\overset{\square}{\varphi} - \varphi\vec{\kappa} \cdot \vec{\calV}_\calM \right) \d \mu_\calM} + \int_{\exbdM} {\Delta \varphi {\calV}_{\exbdM} \d \mu_\exbdM},
\end{equation}
where $\Delta\varphi\left(\bfx,\theta\right)$ on $\exbdM\left[\varphi\right]\left(\theta\right)$ is defined as:
\begin{equation}
	\Delta\varphi\left(\bfx,\theta\right) \coloneqq
	\begin{cases}
		\varphi\left(\bfx,\theta\right), & \text{if }\bfx\in\partial\calM\\
		\varphi^{-}\left(\bfx,\theta\right) - \varphi^{+}\left(\bfx,\theta\right), & \text{if }\bfx\in\Delta\calM\left[\varphi\right]\left(\theta\right)
	\end{cases}.
\end{equation}
Here, $\varphi^{-}\left(\bfx,\theta\right)$ and $\varphi^{+}\left(\bfx,\theta\right)$ are defined as the limits of $\varphi\left(\bfx,\theta\right)$ when approaching $\bfx$ from $-\bfn_{\Delta\calM}\left(\bfx,\theta\right)$ and $\bfn_{\Delta\calM}\left(\bfx,\theta\right)$, respectively. Note that unit normal vectors $\bfn_{\Delta\calM}\left(\bfx,\theta\right)$ and $\bfn_{\exbdM}\left(\bfx,\theta\right)$, the scalar normal velocities $\calV_{\Delta\calM}$ and $\calV_{\exbdM}$, and measures $\mu_{\Delta\calM}$ and $\mu_{\exbdM}$ can be defined in similar ways to $\partial\calM$.

\subsection{Generalization to Vector Parameters}
\label{sec:vector_parameter}
Taking multiple parameters $\btheta=\left(\theta_1...\theta_d \right)$ into account is easily achievable by repeating the formulations for each parameter $\theta_i$. Then $\R^n$ vector velocity terms $v$, $v_{\mathrm{tan}}$, and $\vec\calV$ change to $\R^{n\times d}$ Jacobians, and scalar velocity and derivative terms $\calV$, $\dot\varphi$, and $\overset{\square}{\varphi}$ change to $\R^{1\times d}$ gradients. Then changing the inner product term $\vec{\kappa}\cdot \vec{\calV}_{\calM}$ into a matrix product $\vec{\calV}_{\calM}^T \vec{\kappa}$ from Equations~\eqref{eq:diffint_evol_man} and \eqref{eq:trans_thm_discont} generalizes the trasport theorem for multiple parameters. However, since the transport theorem for multiple parameters is equivalent to enunciating the theorem for each parameter, we keep writing formulations for a single parameter $\theta$ for the sake of simplicity.
