# Supplementary material for: Differentiable Transient Rendering
Source: arXiv:2206.06193 source file (2022-06-13)
Supplement: Supplementary file 2 [file ourmethod-supple.tex]

\section{Derivation Details on Differential Transient Path Integral}
\subsection{Formal Definition of Scene Geometry}
\label{sec:def_scene_geometry}
In physically-based rendering, the scene geometry is usually represented as a 2D manifold, which is unfortunately riddled with discontinuities at the edges of the polygons. To clarify how to treat this discontinuity, we first define piece-wise differentiable manifolds in this section.

The \textit{scene geometry} $\calM$ is a piece-wise differentiable 2D manifold, which satisfies that:
\begin{itemize}
	\item $\calM$ is represented as a finite union of differentiable 2D manifold,s i.e., $\calM=\bigcup_{i=1}^p {\calM_{[i]}}$.
	\item For any two distinct pieces $\calM_{[i]}$ and $\calM_{[j]}$, if they intersect ($\calM_{[i]}\cap\calM_{[j]}\ne \phi$) then the intersection $\calM_{[i]}\cap\calM_{[j]}$ is a differentiable 1D manifold (curve).
\end{itemize}
Then the \textit{boundary of the piece-wise differentiable 2D manifold} $\calM$ is a piece-wise differentiable 1D manifold, defined as $\partial \calM \coloneqq \bigcup_{i=1}^p \partial \calM_{[i]}$, and the \textit{interior of the piece-wise 2D differentiable manifold} $\calM$ is defined as $\Int\calM\coloneqq \calM-\partial\calM=\bigcup_{i=1}^k \Int{\calM_{[i]}}$.
 Note that in usual polygonal representations, each differentiable piece $\calM_{[i]}$ corresponds to each planar polygon (usually triangles), and the boundary of the scene geometry $\partial\calM$ becomes the union of all edges in all polygon meshes. We do not consider self-intersection of scene geometry.

When a point $\bfx$ is in the boundary of the scene $\partial\calM$, we observe that $\bfx$ belongs to one of two cases: it is either contained in exactly one differentiable piece $\partial\calM_{[i]}$, or in the intersection of two differentiable pieces $\partial\calM_{[i]}\cap \partial\calM_{[j]}$. We will call the first case the \textit{boundary edges}, and the second case the \textit{sharp edges} \cite{zhang2019differential,zhang2020path}. Then the boundary of the scene geometry $\partial\calM$ becomes the union of the boundary edges and the sharp edges.

Generally, we can define piece-wise differentiable $m$-manifolds in a similar way, and extend the transport theorem in Equation~\eqref{eq:trans_thm_discont} to piece-wise differentiable manifolds by taking the summation of the equation for each differentiable piece. Then we can use the same equation defining the transport theorem on a piece-wise differentiable $2\left(k+1\right)$-manifold $\Omega_k=\calM^{k+1}$.

\subsection{Product Space Rules}

When an evolving manifold $\mathcal{N}\left(\theta\right)$ is formed as the product of two other evolving manifolds, $\mathcal{N}\left(\theta\right)=\calM_1\left(\theta\right) \times \calM_2\left(\theta\right)$, and there is a scalar function $\varphi\left(\cdot,\theta\right)\colon\mathcal{N}\left(\theta\right)\to\R$ which is the product of scalar functions $\varphi_1\left(\cdot,\theta\right)\colon\calM_1\left(\theta\right)\to\R$ and $\varphi_2\left(\cdot,\theta\right)\colon\calM_2\left(\theta\right)\to\R$, i.e., $\varphi\left(\bfx_1,\bfx_2,\theta\right)=\varphi_1\left(\bfx_1,\theta\right)\varphi\left(\bfx_2,\theta\right)$, we can use the same transport theorem described in Equation~\eqref{eq:trans_thm_discont} by substituting $\calM$ by $\mathcal{N}$. Then Equation~\eqref{eq:trans_thm_discont} can be evaluated in terms of $\calM_1$ and $\calM_2$ as follows:
\begin{align}
	\label{eq:transport_thm_product_space}
	\begin{split}
		\overset{\square}{\varphi}\left(\bfx_1,\bfx_2,\theta\right) =& \overset{\square}{\varphi}_1\left(\bfx_1,\theta\right)\varphi_2\left(\bfx_2,\theta\right)
		+ \varphi_1\left(\bfx_1,\theta\right)\overset{\square}{\varphi}_2\left(\bfx_2,\theta\right)\\
		\vec\kappa_{\mathcal{N}}\left(\bfx_1,\bfx_2,\theta\right) =& \left(\vec\kappa_{\calM_1}\left(\bfx_1,\theta\right), \vec\kappa_{\calM_2}\left(\bfx_2,\theta\right)\right), \\
		\vec{\calV}_{\mathcal{N}}\left(\bfx_1,\bfx_2,\theta\right) =& \left(\vec{\calV}_{\calM_1}\left(\bfx_1,\theta\right), \vec{\calV}_{\calM_2}\left(\bfx_2,\theta\right)\right), \\
		\partial\overline{\mathcal{N}}\left[\varphi\right]\bratheta =& \partial\overline{\calM_1}\left[\varphi_1\right]\bratheta\times\calM_2\bratheta \cup \calM_1\bratheta \times \partial\overline{ \calM_2}\left[\varphi_2\right]\bratheta, \\
		\Delta\varphi\left(\bfx_1,\bfx_2,\theta\right) =& \begin{cases}
			\varphi_2 \Delta\varphi_1 & \text{if }\left(\bfx_1,\bfx_2\right)\in\partial\overline{\calM_1}\times\calM_2 \\
			\varphi_1 \Delta\varphi_2 & \text{if }\left(\bfx_1,\bfx_2\right)\in\calM_1 \times \partial\overline{\calM_2}
		\end{cases}, \\
		\calV_{\overline{\partial\mathcal{N}}}\left(\bfx_1,\bfx_2,\theta\right) =& \begin{cases}
			\varphi_2 \calV_{\exbdM_1} & \text{if }\left(\bfx_1,\bfx_2\right)\in\partial\overline{\calM_1}\times\calM_2 \\
			\varphi_1\calV_{\exbdM_2} & \text{if }\left(\bfx_1,\bfx_2\right)\in\calM_1 \times \partial\overline{\calM_2}
		\end{cases}.
	\end{split}
\end{align}
These rules can be extend in a similar way to an arbitrary number of products, such as the order-$k$ path space $\Omega_k=\calM^{k+1}$.

\subsection{Terms in the Path Integral}

Recall the transient path integral, the path throughput, and the correlated importance described in the main paper, respectively, for negligible scattering delays surface path vertices:
\begin{gather}
	\label{eq:trans_pathintegral}
	I= \int_\Omega{
		f_{\calT}\left(\bar \bfx  \right)
		\d \mu\left(\bar \bfx\right)}, \\
	f_{\calT}\left(\bar{\bfx}\right) \coloneqq \mathfrak{T}\left(\sPath\right) S_e\left(\sPath\right), \\
	\mathfrak{T}\left(\sPath\right) \coloneqq \left[
	\prod_{i=1}^{k-1}\rho\left( \bfx_{i-1}, \bfx_i,\bfx_{i+1} \right)
	\right]\left[
	\prod_{i=0}^{k-1}G\left(\bfx_i, \bfx_{i+1}\right) V\left(\bfx_i,\bfx_{i+1}\right)
	\right], \\
	S_e\left(\sPath\right) = \int_{-\infty}^{\infty}{
		L_e \left(\bfx_0 ,\bfx_1,t\right)
		W_e \left(\bfx_{k-1} ,\bfx_k,t+\tof\left(\bar\bfx\right)\right)
	\d t}.
\end{gather}

For a mathematically rigorous derivation, we define each term in the path integral: $L_e$, $\rho$, $W_e$, $G$, and $V$.
\begin{definition}
	\label{def:gterm}
	For given scene geometry $\calM$, the geometric function $G\colon \Int\calM \times \Int\calM \to \R$ is defined as:
	\begin{equation}
		\label{eq:def_gterm}
		G\left(\bfx,\bfy\right) \coloneqq
		\begin{cases}
			\frac{
				\abs{\hn_\bfx \cdot \homega_{\bfx\bfy}} \abs{\hn_\bfy \cdot \homega_{\bfy\bfx}}
			}{
				\norm{\bfx-\bfy}^2
			} & \bfx\ne \bfy \\
			0 & \bfx=\bfy
		\end{cases}.
	\end{equation}
\end{definition}
Also, when the domain is restricted to differentiable pieces of the scene geometry, denoted by $\Int{\calM_{[i]}}\times\Int{\calM_{[j]}}$ ($1\le i,j\le p$), then the restricted function can be continuously extended onto $\calM_{[i]}\times\calM_{[j]}$, which contains their boundaries $\partial\calM_{[i]}$ and $\partial\calM_{[j]}$. We will denote this function as $\evalat{G}{\calM_{[i]}\times\calM_{[j]}}\colon \calM_{[i]}\times\calM_{[j]}\to\R$, where $\evalat{G}{\calM_{[i]}\times\calM_{[j]}}$ is a continuous function. Note that the entire geometric function $G$ satisfies $\Delta\left(\calM^2 \right)\left[G\right]=\partial\left(\calM^2\right)$.

\begin{definition}
	\label{def:visi}
	For given scene geometry $\calM$, the visibility function $V\colon\calM\times\calM\to\R$ is defined as:
	\begin{equation}
		\label{eq:def_visi}
		V\left(\bfx,\bfy\right)\coloneqq
		\begin{cases}
			1 & \mathrm{openlineseg}\left(\bfx,\bfy\right)\cap\calM=\phi\\
			0 & otherwise
		\end{cases},
	\end{equation}
\end{definition}
\noindent where $\mathrm{openlineseg}\coloneqq\left\{\lambda \bfx+\left(1-\lambda\right)\bfy\mid0<\lambda<1\right\}$ means the open line segment between  two given points.
Unlike the geometric function $G$ and the visibility function $V$, the light source emission function $L_e$, surface scattering function (BSDF) $\rho$, and the sensor sensitivity function $W_e$ vary depending on the scene. We can introduce the following conditions which those terms should satisfy in practice:

\begin{enumerate}[\text{A}.1]
	\item For any fixed $\bfx_0,\bfx_1\in\calM$, $L_e\left(\bfx_0\to\bfx_1,\cdot\right)\colon\R\to\R$ as a function of $t$ contains a finite number of jump discontinuities at $t_{L1}...t_{Lq}$ and a finite number of Dirac delta distributions at $t_1...t_r$. Except for $t_{L1}...t_{Lq}$ and $t_1...t_r$, $L_e\left(\bfx_0\to\bfx_1,\cdot\right)$ is continuous. Also, $t_{L1}...t_{Lq}$ and $t_1...t_r$ vary continuously when $\bfx_0$ and $\bfx_1$ vary continuously.
	\label{enum:A1}
	
	\item For any fixed $\bfx_{N-1},\bfx_N\in\calM$, $W_e\left(\bfx_{N-1}\to\bfx_N,\cdot\right)\colon\R\to\R$ as a function of $t$ contains a finite number of jump discontinuities at $t_{W1}...t_{Ws}$. Except for $t_{W1}...t_{Ws}$, $W_e\left(\bfx_0\to\bfx_1,\cdot\right)$ is continuous. Also, $t_{W1}...t_{Ws}$ vary continuously when $\bfx_0$ and $\bfx_1$ vary continuously.
	\label{enum:A2}
	
	\item The source emission $L_e$ does not have non-zero energy on spatially zero-measure sets.
	\label{enum:A3}
	
	\item The scattering function $\rho$ does not contain a Dirac delta, i.e., there is no ideal specular reflection, and is continuous except when the incoming or outgoing directions are perpendicular to the surface normal.
	\label{enum:A4}
\end{enumerate}

\ref{enum:A1} and \ref{enum:A2} are our novel assumptions for transient rendering, while \ref{enum:A3} and \ref{enum:A4} are  common assumptions used in physically-based differentiable rendering~\cite{li2018differentiable, loubet2019reparameterizing, zhang2020path, bangaru2020unbiased, zhang2019differential}. Note that these assumptions cover most of practical cases.

\subsection{Differential Transient Path Integral}

To differentiate Equation~\eqref{eq:trans_pathintegral} using the transport theorem in Equation~\eqref{eq:trans_thm_discont}, we will first evaluate the boundary path space $\bdps\left[f_{\calT}\right]\left(\theta\right)$. For simplicity, we first fix $k$ and evaluate the order-$k$ boundary path space $\bdpsk$. By definition of extended boundary (Equation~\eqref{eq:def_exbd}), $\bdpsk$ consists of the (geometric) boundary $\partial\Omega_k$ and the discontinuity set $\Delta\Omega_k\left[f_{\calT}\right]$. Since the total throughput $f_{\calT}$ is the product of partial terms $S_e$, $\rho$, $V$, and $G$, the entire discontinuity set can be represented as the union of discontinuity sets caused by each of those partial terms as follows:
\begin{align}
	\label{eq:total_exbd_union}
	\begin{split}
		\bdpsk\left[\ftau\right] =& \partial\Omega_k \cup\Delta\Omega_k\left[\ftau\right] \\
		=& \partial\Omega_k
		\cup \Delta\Omega_k\left[S_e\right]
		\cup \Delta\Omega_k\left[G_1 \cdots G_k\right] \\
		&\cup \Delta\Omega_k\left[V_1 \cdots V_k\right]
		\cup \Delta\Omega_k\left[\rho_1 \cdots \rho_{k-1}\right].
	\end{split}
\end{align}
Note that both boundary edges and sharp edges are contained in $\partial\Omega_k$ as mentioned in \S\ref{sec:def_scene_geometry}. 

Applying the product space rule Eq.~\eqref{eq:transport_thm_product_space} to Eq.~\eqref{eq:total_exbd_union}, $\Delta\Omega_k\left[G_1 \cdots G_k\right]$, $\Delta\Omega_k\left[V_1 \cdots V_k\right]$, and $\Delta\Omega_k\left[\rho_1 \cdots \rho_{k-1}\right]$ can be rewritten as follows:
\begin{align}
	\label{eq:exbd_product_rule}
	\small
	\begin{split}
		\Delta\Omega_k\left[G_1 \cdots G_k\right] =& \bigcup_{i=1}^{k} \calM_0 \times\cdots\calM_{i-2}\times \Delta\calM^2\left[G\right]
		\times \calM_{i+1}\times\cdots\calM_k, \\
		\Delta\Omega_k\left[V_1 \cdots V_k\right] =& \bigcup_{i=1}^{k} \calM_0 \times\cdots\calM_{i-2}\times \Delta\calM^2\left[V\right]
		\times \calM_{i+1}\times\cdots\calM_k, \\
		\Delta\Omega_k\left[\rho_1 \cdots \rho_{k-1}\right] =& \bigcup_{i=1}^{k-1} \calM_0 \times\cdots\calM_{i-2}\times \Delta\calM^3\left[\rho\right]
		\times \calM_{i+2}\times\cdots\calM_k .
	\end{split}
\end{align}

\paragraph{Vanishing and overlapping discontinuities}
Some discontinuity sets of partial terms, $\Delta\Omega_k\left[S_e\right]$, $\Delta\calM^2\left[G\right]$, $\Delta\calM^2\left[V\right]$, and $\Delta\calM^3\left[\rho\right]$ may not contribute to the total discontinuity set.
As discussed in previous work~\cite{zhang2020path}, $\Delta\calM^3\left[\rho\right]$ is caused at the horizontal ray direction, but in that case the geometric term $G$ is continuously zero. For a formal mathematical analysis we rely on the following proposition:
\begin{proposition}
	\label{prop:conti_zero}
	Given a set $X\in \R^n$ and a subset $A\subset X$, suppose that a function $\varphi_1\colon X\to \R$ is continuously zero on $A$ and a function $\varphi_2\colon X\to\R$ is a bounded function. Then even if $\varphi_2$ is discontinuous in $A$, $A$ does not contribute to the discontinuity set of $\varphi_1\varphi_2$, i.e., $A\cap \Delta X\left[\varphi_1 \varphi_2\right]=\phi$.
\end{proposition}

Thus, we can omit $\Delta\Omega_k\left[\rho_1\cdots\rho_{k-1}\right]$ from Equation~\eqref{eq:total_exbd_union}. The visibility function $V$ also presents a discontinuity at the horizontal ray direction, which vanished by the geometric function $G$. Then Equation~\eqref{eq:total_exbd_union} can be rewritten in the following simpler form: 

\begin{align}
	\label{eq:total_exbd_union_minimal}
	\begin{split}
		\partial\overline{\Omega}_k \left[\ftau\right]
		=& \partial\Omega_k
		\cup \Delta\Omega_k\left[S_e\right] \\
		&\cup\left(\Delta\Omega_k\left[G_1 V_1 \cdots G_k V_k\right]-\partial\Omega_k\right).
	\end{split}
\end{align}
Note that in the last term of Equation~\eqref{eq:total_exbd_union_minimal} we will evaluate the discontinuity set of the product term $GV$ directly, without considering discontinuities on $\partial\Omega_k$, already accounted for in the first term of Equation~\eqref{eq:total_exbd_union_minimal}.

\subsubsection{Discontinuity of $GV$ terms}
The term $(\Delta\Omega_k\left[G_1 V_1 \cdots G_k V_k\right]-\partial\Omega_k)$ caused by silhouette edges can be represented by the product rule (Equation~\eqref{eq:transport_thm_product_space}) as:
\begin{align}
	\label{eq:disconti_GV_term_path}
	\begin{split}
		\Delta\Omega_k\left[G_1 V_1 \cdots G_k V_k\right]&-\partial\Omega_k
		= \bigcup_{i=1}^{k} \calM_0 \times\cdots\calM_{i-2} \\
		&\times \left( \Delta\calM^2\left[GV\right]-\partial{\calM}^2 \right)
		\times \calM_{i+1}\times\cdots\calM_k,
	\end{split}
\end{align}
where the term $\left(\Delta\calM^2\left[GV\right]-\partial{\calM}^2 \right)$  is obtained by the following lemma:

\begin{lemma}
	\label{lem:disconti_GV}
	The discontinuity submanifold of GV can be specified as:
	\begin{align}
		\label{eq:disconti_GV_term_mani}
		\begin{split}
			\Delta\calM^2\left[GV\right]-\partial{\calM}^2
			=& \Delta\left(\Int{\calM^2}\right)\left[GV\right] \\
			=&\{ \left(\bfx,\bfy\right)\in \Int{\calM^2)} \mid 
			\normalfont\text{line segment between }\bfx,\bfy \\
			& \normalfont\text{only intersects silhouette edges of }\calM\}. \\
		\end{split}
	\end{align}
\end{lemma}

A line segment between $\left(\bfx,\bfy\right)$ intersects a silhouette edge of $\calM$ if and only if: 
\begin{align}
	\begin{split}
		\exists \bfz\in&\mathrm{openlineseg}\left(\bfx,\bfy\right)\cap \calM \text{ s.t. one of the three cases holds:}\\
		& \bfz\in\Int\calM\text{ and }\bfn\left(\bfz\right)\cdot\left(\bfy-\bfx\right)=0,\\
		& \bfz\in\partial\calM_{[i]}\text{ (boundary edge), or} \\
		& [\bfz\in\partial\calM_{[i]}\cap\partial\calM_{[j]}\text{ with }{[i]}\ne j\text{ (sharp edge) and} \\
		&\left(\bfn_i\left(\bfz\right)\cdot{\bfy-\bfx}\right) \left(\bfn_j\left(\bfz\right)\cdot\left(\bfy-\bfx\right)\right)\le 0].
	\end{split}
\end{align}

To prove the lemma,  we first show that $V^{-1}\left(\left\{1\right\}\right)\cap\Int{\calM^2}\subset \Intc{\calM^2}\left[GV\right]$, i.e. for any pair of mutually visible points $\left(\bfx,\bfy\right)\in\Int{\calM^2}$ with $V\left(\bfx,\bfy\right)=1$, $GV$ is continuous on $\left(\bfx,\bfy\right)$. If $\bfy-\bfx$ is orthogonal to $\bfn\left(\bfx\right)$ or $\bfn\left(\bfy\right)$, the claim holds since $G$ is continuously zero on $\left(\bfx,\bfy\right)$. Otherwise, we can easily observe that the visible pair of points are still visible when they move within a sufficiently small distance.

Second, we show that if $\left(\bfx,\bfy\right)\in V^{-1}\left(\left\{0\right\}\right)\cap\Int{\calM^2}$ and the line segment between them intersects a point $z\in\calM$ which is not on a silhouette edge, then $V$ is continuous on $\left(\bfx,\bfy\right)$.  
Note that by definition of silhouette described in Lemma~\ref{lem:disconti_GV}, $\bfz$ belongs to one of  two cases: i) $\bfz\in\Int\calM$ and $\bfn\left(\bfz\right)\cdot\left(\bfy-\bfx\right)$, or ii) $\bfz\in\partial\calM_{[i]}\cap\partial\calM_{[j]}$ with $i\ne j$ (sharp edge) and $\left(\bfn_i\left(\bfz\right)\cdot{\bfy-\bfx}\right) \left(\bfn_j\left(\bfz\right)\cdot\left(\bfy-\bfx\right)\right)> 0$. In both cases, the line segment penetrates the open disk which neighbors $\bfz$. Then we observe that when $\bfx$ and $\bfy$ moves within a sufficiently small distance, the line segment between them still penetrates the open disk.

\subsubsection{Discontinuities of the $S_e$ term}
Recall the assumptions \ref{enum:A1} and \ref{enum:A2} for source emission $L_e$ and sensor sensitivity $W_e$. Given $\bfx_0$ and $\bfx_1$, $L_e\left(\bfx_0\to\bfx_1,\cdot\right)$ has Dirac delta mass at $t=t_{L1}...t_{Lj}$, and given $\bfx_{k-1}$ and $\bfx_k$, $W_e\left(\bfx_{k-1}\to\bfx_k,\cdot\right)$ has discontinuity at $t=t_{W1}...t_{Wk}$. By the following lemma, we can obtain the discontinuity of $S_e$.

\begin{lemma}
	\label{lem:disconti_Se}
	With assumptions \ref{enum:A1} and \ref{enum:A2}, the discontinuity of $S_e$ can be determined as:
	\begin{align}
		\label{eq:disconti_Se_term}
		\begin{split}
			\Delta\Omega_k\left[S_e\right]
			= \{
			\bar\bfx\in\Omega_k \mid& \tof\left(\bar\bfx\right)=t_{Wi}-t_{j} \\
			&\normalfont\text{ for some }1\le i \le s,\ 1\le j \le r
			\}.
		\end{split}
	\end{align}
\end{lemma}

Note that this representation does not include a vanishing part for $G=0$. To prove this lemma, first let $u_{t_0}\left(t\right)$ denote the unit step function, which is defined as $u_{t_0}\left(t\right)=1$ for $t>t_0$ and $u_{t_0}\left(t\right)=0$ otherwise. Also, $\delta_{t_0}\left(t\right)$ denotes the Dirac delta function centered at $t_0$ so that $\delta_{t_0}\left(t\right)=\delta\left(t-t_0\right)$. Important facts to prove Lemma~\ref{lem:disconti_Se} is that $u_{t_0}\star u_{t_1}$ is a continuous function and $\delta_{t_0}\star u_{t_1}=u_{t_1-t_0}$, where $\star$ denotes the cross-correlation. Since $S_e\left(\bfx_0,\bfx_1,\bfx_{k-1},\bfx_k, t=\tof\left(\sPath\right)\right)$ is the correlation of $L_e$ and $W_e$ in the temporal domain, the only discontinuity occurs when $\tof\left(\sPath\right)$ lies on the discontinuous point of $\delta_{t_j}\star u_{t_{Wi}}$.

For example, suppose that the source is $L_e\left(\bfx_0,\bfx_1,t\right)=L_e\left(\bfx_0,\bfx_1\right)\delta\left(t\right)$ and the sensor is $W_e\left(\bfx_{N-1},\bfx_N,t\right)=W_e\left(\bfx_{k-1},\bfx_k\right)$ $\mathrm{box}\left(t;t_\text{start}, t_\text{end}\right)$ where $\mathrm{box}\left(t;t_\text{start}, t_\text{end}\right)$ refers to the unit box function starting from $t_\text{start}$ and ending at $t_\text{end}$. In this case the discontinuity of $S_e$, $\Delta\Omega_k\left[S_e\right]$, is the set of paths with travel time $t_\text{start}$ or $t_\text{end}$. In practice, if the light source and the sensor are not Dirac deltas then $\Delta\Omega_k\left[S_e\right]=\phi$. %

\paragraph{Boundary Contribution $\Delta \ftau$ and Normal Velocities $\calV_{\bdps_k}$}
When $\Delta\Omega_k\left[S_e\right]$ becomes an empty set, the boundary path space $\bdps_k$ consists of $\partial\Omega_k$ and $\Delta\Omega_k\left[G_1 V_1 \cdots G_k V_k\right]-\partial\Omega_k$. For a global parameterization we only need to concern ourselves with  the discountinuity of the $GV$ term $\Delta\Omega_k\left[G_1 V_1 \cdots G_k V_k\right]-\partial\Omega_k$. Then the discontinuity comes from the visibility, so $\Delta\ftau$ becomes the same as $\ftau$ and the normal velocity $\calV_{\bdps_k}$ converges to its steady-state counterpart.
