# Supplementary material for: Differentiable Transient Rendering
Source: arXiv:2206.06193 source file (2022-06-13)
Supplement: Supplementary file 3 [file appendix.tex]

\appendix
\section{Appendix}
\label{appendix}

\subsection{Detail of the Interior Integral Term}
\label{appendix_formulae}
\NEW{
The normal derivative of the light throughput $\dnT\left(\sPath\right)$ is obtained by the product rule:
	\begin{equation}\small
		\label{eq:deriv_throughput}
		\dnT(\sPath) = \sum_{j=1}^{k-1}\left[
			\dn{\rho}_j	\prod_{\substack{i=1\\i \ne j}}^{k-1}\rho_i+\prod_{i=0}^{k-1} G_i V_i
		\right]+\sum_{j=0}^{k-1}\left[
			\prod_{i=1}^{k-1}\rho_i + \left(\dn{G}_j V_j + G_j \dn{V}_j \right) \prod_{\substack{i=0\\i \ne j}}^{k-1} G_i V_i
		\right], 
	\end{equation}
	where
	\begin{equation}
		\begin{split}
			\rho_i=\rho\left(\bfx_{i-1}\to\bfx_i\to\bfx_{i+1}\right), \\ \nonumber
			G_i = G\left(\bfx_i \lrarrow \bfx_{i+1}\right), \\ \nonumber
			V_i = V\left(\bfx_i \lrarrow \bfx_{i+1}\right), \nonumber
		\end{split}
	\end{equation}
	for any index $i$.

	Note that the normal derivative also satisfies common differentiation rules such as the product rule, $\left[\varphi_1\left(\sPath\right) \varphi_2 \left(\sPath\right)\right]^\square =\overset{\square}{\varphi_1}\left(\sPath\right){\varphi_2}\left(\sPath\right)+{\varphi_1}\left(\sPath\right)\overset{\square}{\varphi_2}\left(\sPath\right)$,
	or the composition rule, $\left[\varphi_3\left(\varphi_1\left(\sPath\right)\right)\right]^\square =\overset{\square}{\varphi_3}\left(\varphi_1\left(\sPath\right)\right) \overset{\square}{\varphi_1}\left(\sPath\right)$ 
	as well as conventional derivatives $\left[\varphi_1\left(\sPath\right) \varphi_2 \left(\sPath\right)\right]^\cdot$ or $\left[\varphi_3\left(\varphi_1\left(\sPath\right)\right)\right]^\cdot$ do. Here,
	$\varphi_1$, $\varphi_2$, and $\varphi_3$ can be arbitrary functions.

	The normal derivative of the correlated importance $\dnSe\left(\sPath\right)$ can be expressed in terms of  partial derivatives $\pfrac{S_e\left(\sPath\right)}{t}$ and $\pfrac{S_e \left(\sPath\right)}{\bfx_i}$ for $i=0,1,k-1,k$ in Equation~\eqref{eq:diff_Se_twoterms}. Here, these partial derivatives are determined based on considering $S_e$ as a function of $t$, $\bfx_0$, $\bfx_1$, $\bfx_{k-1}$, and $\bfx_k$. Concretely, each partial derivatives can be evaluated as follows:
	\begin{equation}
		\label{eq:Se_5partials}
		\small
		\begin{split}
			\pfrac{S_e\left(\sPath\right)}{t}=&
			\int_{-\infty}^{\infty}\biggl[{
				\pfrac{L_e}{t}\left(\bfx_0,\bfx_1,t'\right)W_e \left(\bfx_{k-1},\bfx_k,t'+t\right)} \\
			&\quad\quad+L_e\left(\bfx_0,\bfx_1,t'\right)\pfrac{W_e}{t} \left(\bfx_{k-1},\bfx_k,t'+t\right)
			\biggl] \d t'\bigg|_{t=\tof\left(\sPath\right)}, \\
			\pfrac{S_e\left(\sPath\right)}{\bfx_i} =& \left.\int_{-\infty}^{\infty}{
				\pfrac{L_e}{\bfx_i}\left(\bfx_0,\bfx_1,t'\right)W_e \left(\bfx_{k-1},\bfx_k,t'+t\right)
			\d t'}\right|_{t=\tof\left(\sPath\right)}\text{ for }i=0,1,\\
			\pfrac{S_e\left(\sPath\right)}{\bfx_i} =& \left.\int_{-\infty}^{\infty}{
				L_e\left(\bfx_0,\bfx_1,t'\right)\pfrac{W_e}{\bfx_i} \left(\bfx_{k-1},\bfx_k,t'+t\right)
			\d t'}\right|_{t=\tof\left(\sPath\right)}\text{ for }i=k-1,k.
		\end{split}
	\end{equation}
}
